# Supplementary material for: Removal Attack and Defense on AI-generated Content Latent-based Watermarking
Source: arXiv:2509.11745 source file (2025-11-12)
Supplement: Supplementary file 1 [file changes_appendix.tex]

\section{Changes Made}


\subsection{Main Changes Made}

\color{blue}
These changes are highlighted in blue in the main text.
\subsubsection{Expanded Evaluation Scope}
Besides the existing evaluation on SD 2.1, we have performed further evaluations of the proposed stealthy attack and boundary-hiding defense on SD 1.6 and SD XL in Section \ref{appendix:eval}. We have also updated our code repository in Section \ref{appendix:code} to include the additional models. 
Our empirical evaluations on SD2.1 shows that both our proposed attack and defense generalizes to other LDMs with different architectures and larger latent space dimensions. As the evaluation results for SD 1.6 and SD 2.1 are similar (due to the same latent-space dimensions and similar architectures), we have omitted the results from the text due to space constraints. 


\subsubsection{Approximation of Secret Transformation}
In Section~\ref{section:defense}, we established that the defense is secure against a \textit{known watermark attack}. However, in Section~\ref{discussion:known_watermark_boundary}, we introduced and considered a more powerful adversary threat model, known as the {known boundary attack}. While we do not know the precise method by which this attack would be implemented, we outline the general strategy such an adversary might employ to approximate the secret transformation. This discussion highlights potential vulnerabilities of the defense under stronger adversarial assumptions and suggests directions for future analysis.

\subsubsection{Scalability of Defense}

While Section~\ref{section:defense} characterized the security requirements for our defense through Condition~\ref{condition:transformation}, the reviewers noted that the proposed construction suffers from scalability issues due to the $O(d^2)$ complexity of multiplying a $d \times d$ orthonormal matrix with a $d$-dimensional vector.
In Section~\ref{discussion:scalability},  we discuss possible methods to improve the scalability of our defense. Our approach involves selecting $T$ from certain classes of transformations that both satisfy Condition~\ref{condition:transformation} and admit efficient matrix-vector multiplication. This allows us to maintain security while significantly reducing the computational overhead in practical implementations. 

\subsubsection{Study on Image Quality Post-Attack}
In Section \ref{appendix:additional_img}, we have included additional pairs of images for readers to assess the perceptual and semantic similarity of the image pairs, together with a link to an anonymized repository with $10,000$ image pairs. 



\subsubsection{Relaxing Condition \ref{condition:transformation}}
In our previously submitted version, Condition \ref{condition:transformation} states two requirements, namely
\begin{enumerate}
    \item The current condition stated in  Condition \ref{condition:transformation}, and
    \item The distribution of both random variables $T|(Y_1,\dots,Y_m)$ and $T$ must be the same. 
\end{enumerate}
However, we have since strengthened our analysis by showing that the second condition is actually implied by the first (Lemma \ref{lemma:1b}). This simplification is significant because it makes Condition~\ref{condition:transformation} easier to verify for specific classes of transformations. Consequently, when identifying efficient transformation classes in Section~\ref{discussion:scalability}, we need only check the first condition. 

\subsubsection{Latent Space Attacks and Defense Emphasis}
Reviewers questioned the motivation for latent space attacks, which we address in the introduction by highlighting their theoretical and practical relevance. We have also strengthened the emphasis on our paper's primary contribution: proposing a defense mechanism specifically designed to protect against latent space-based adversarial attacks.

\color{black}
\subsection{Minor Changes Made}
The minor changes made here clarifies some points made by reviewers, and cosmetic changes. 
\subsubsection{Why AC2 and 3 Outperforms AC1}
In Section~\ref{section:eval_sd2.1}, we include a brief discussion explaining why AC2 and AC3 outperform AC1, under the heading ``Improved Attack Performance in AC2 and AC3''. This performance gap arises because the watermark detector's extraction process involves inverting the latents before performing the attack, which aligns with the method employed by AC2 and AC3.

\subsubsection{Cosmetic Changes}
We have also made minor cosmetic improvements throughout the paper in terms of presentation and language, and made some of the proofs more concise when possible. 
